# Supplementary material for: Temporal Convolutional Networks for Action Segmentation and Detection
Source: arXiv:1611.05267 source file (2016-11-16)
Supplement: Supplementary file 1 [file appendix.tex]

\section{Supplemental Material}

\subsection{Additional Datasets}

\textbf{JHU-ISI Gesture and Skill Assessment Working Set (JIGSAWS) ~\cite{JIGSAWS}}
was introduced to improve quantitative evaluation of robotic surgery training tasks. 
%While JIGSAWS includes data for three unique training tasks, 
We used Leave One User Out cross validation on the suturing activity, which consists of 39 sequences performed by 8 users about 5 times each. The dataset includes video and synchronized robot kinematics (position, velocity, and gripper angle) for each robot end effector as well as corresponding action labels with 10 action classes. Sequences are a few minutes long and typically contain around 20 action instances.

% \textbf{Georgia Tech Egocentric Activities (GTEA)~\cite{fathi_cvpr_2011}}
% contains 28 videos of 7 kitchen activities including making a sandwich and making coffee. For each of the four subjects, there is one instance of each activity.
% The camera is mounted on the head of the user and is pointing at the area in front them. 
% On average there are about 30 actions per video and videos are around a minute long. We used the 11 action classes defined in~\cite{fathi_iccv_2011} and evaluated using leave one user out. We show results for user 2 to be consistent with \cite{fathi_iccv_2011} and \cite{singh_cvpr_2016b}.

\begin{table*}[t]
	\centering

    	\begin{tabular}{ccc}
		%		 &  \\
		% -----------Salads----------
		\begin{tabular}{| l | c | c |}
			\multicolumn{3}{c}{50 Salads (``eval'' setup)}\\
			\hline
			\textbf{Sensor-based}  & \textbf{Edit} & \textbf{Acc}\\
			\hline      
			%           \cite{lea_icra_2016} LC-SC-CRF*  & 58.0 & 81.7 \\
			LC-SC-CRF \cite{lea_icra_2016}   & 50.2 & 77.8      \\  
			%           \cite{lea_icra_2016} LC-SC-CRF   &  &       \\
			LSTM & 54.5 & 73.3\\            
			%Framewise (not segmental)
			%LSTM (segmental)  & 51.25 & 69.80\\ 
			%\hline
			%tCNN (framewise)  & 45.67 & 82.12\\ 
			%           \cite{lea_eccv_2016} ST-CNN + Seg & 55.5 & 82.1 \\ 
			%           TCN  & \textbf{75.5} & \textbf{84.2}\\
			TCN   & \textbf{65.6} & \textbf{82.0}\\         
			%           TCN (ours) & \textbf{72.5} & \textbf{89.6}\\
			\hline
			\textbf{Video-based} & \textbf{Edit} & \textbf{Acc} \\
			\hline
			%sCNN (framewise)  & 24.10 & 66.64\\ 
			%stCNN (framewise)  & 49.6 & 69.35\\ 
			VGG \cite{lea_eccv_2016}  & 7.6
			& 38.3 \\           
			IDT \cite{lea_eccv_2016}  & 16.8 & 54.3
			\\
			Seg-ST-CNN \cite{lea_eccv_2016}  & \textbf{62.0} & 72.0\\ 
			%           TCN  & \textbf{65.1} & \textbf{72.4}\\\
			%           \hline
			Spatial CNN & 28.4  & 68.6 \\
			ST-CNN & 55.5 & 74.2 \\                             
			TCN  & 61.1 & \textbf{74.4}\\
			%           TCN (ours) & \textbf{78.5} & \textbf{83.7}\\            
			\hline
		\end{tabular}&
		\begin{tabular}{| l | c | c |}
			\multicolumn{3}{c}{GTEA}\\
			\hline
			\textbf{Video-based} & \textbf{Edit} & \textbf{Acc} \\
			\hline
			Hand-crafted \cite{fathi_iccv_2011}& - & 47.7  \\          
			EgoNet \cite{singh_cvpr_2016b}& - & 57.6  \\               
			TDD \cite{singh_cvpr_2016b}& - & 59.5 \\
			EgoNet+TDD \cite{singh_cvpr_2016b}& - & \textbf{68.5} \\           
			%           \cdashline{1-3}
			Spatial CNN  & 36.6 & 56.1  \\
			ST-CNN  & 53.4 & 64.5 \\            
			%           TCN & \textbf{64.2} & 63.4  \\
			TCN & \textbf{58.8} & 66.1  \\
			\hline
		\end{tabular}       
		&
		\begin{tabular}{| l | c | c |}
			\multicolumn{3}{c}{JIGSAWS}\\
			\hline
			\textbf{Sensor-based}  & \textbf{Edit} & \textbf{Acc} \\
			\hline 
			LSTM \cite{dipietro_miccai_2016} & 75.3 & 80.5\\           
			LC-SC-CRF \cite{lea_icra_2016}& 76.8 & \textbf{83.4}\\
			Bidir LSTM\cite{dipietro_miccai_2016}  & 81.1 & 83.3\\ 
			SD-SDL\cite{Stefati_m2cai_2015} & 83.3  & 78.6 \\
			%           TCN \TODO{old. fix?}  & \textbf{89.3} & 82.4\\
			TCN  & \textbf{85.8} & 79.6\\           
			
			\hline 
			
			\textbf{Vision-based }  & \textbf{Edit} & \textbf{Acc}\\
			\hline
			MsM-CRF  \cite{tao_miccai_2013}& -& 71.7 \\            
			IDT \cite{lea_eccv_2016} & 8.5 & 53.9 \\
			VGG \cite{lea_eccv_2016} & 24.3 & 45.9  \\                 
			%sCNN (framewise)  & 17.44 & 57.80\\ 
			%stCNN (framewise)  & 71.23 & 74.59\\ 
			Seg-ST-CNN \cite{lea_eccv_2016}&  66.6 & 74.7\\ 
			%           \cite{lea_iros_2016} LC-CR-CRF &  - & 76.XX \\ 
			%           TCN (ours) & \textbf{85.6} & \textbf{78.3}\\
			%           \hline
			Spatial CNN & 37.7 & 74.0\\
			ST-CNN & 68.0 & 77.7\\
			TCN  & \textbf{83.1} & \textbf{81.4}\\          
			\hline
		\end{tabular}
	\end{tabular}

	\caption{ Results on 50 Salads, Georgia Tech Egocentric Activities, and  JHU-ISI Gesture and Skill Assessment Working Set. Notes: (1) Results using VGG and Improved Dense Trajectories (IDT) were intentionally computed without a temporal component for ablative analysis, hence their low edit scores. (2) We re-computed~\cite{lea_icra_2016} using the author's public code to be consistent with the setup of~\cite{richard_cvpr_2016}.}
	\label{table:results}
\end{table*}
